# Supplementary material for: Control of concerted back-to-back double ionization dynamics in helium
Source: arXiv:2005.10880 ancillary file (2021-10-11)
Supplement: Supplementary file 1 [file ESI.pdf]

# Supporting Information for:
# Control of concerted back-to-back double ionization dynamics in helium

Henrik R. Larsson*
*Institut für Physikalische Chemie, Christian-Albrechts-Universität zu Kiel, Olshausenstraße 40, 24098 Kiel, Germany and Department of Chemical Physics, Weizmann Institute of Science, 76100 Rehovot, Israel*

David J. Tannor
*Department of Chemical Physics, Weizmann Institute of Science, 76100 Rehovot, Israel*
(Dated: May 21, 2020)

## CONTENTS

A. Numerical Details 1
1. Local Control 1
a. "Simple man" optimization 1
b. Parameters 2
2. Derivative-free optimization 2
3. Krotov Optimization 2
4. Control of classical dynamics 2
5. Simulation Method: Dynamically pruned discrete variable representation (DP-DVR) 3

B. Further results for optimization using the Krotov algorithm 3

References 4

## Appendix A: Numerical Details

In the following, numerical details and parameters will be presented for the various control procedures and for the simulation.

### 1. Local Control

We first detail the second-order expression for local control. This is needed if the operator $\hat{O}$ does not interact with $\hat{X}$ to first order, i.e., $[\hat{X}, \hat{O}]$ vanishes. In that case, the second-order time-derivative of $\langle\hat{O}\rangle$ has to be considered:

$$\begin{aligned}\frac{\mathrm{d}^2\langle\hat{O}\rangle}{\mathrm{d}t^2} =& -\langle[[\hat{O},\hat{H}_0],\hat{H}_0]\rangle - \mathrm{i}\frac{\mathrm{d}A(t)}{\mathrm{d}t}\langle[\hat{O},\hat{X}]\rangle \\ &- A(t)\left\{\langle[[\hat{O},\hat{H}_0],\hat{X}]\rangle + \langle[[\hat{O},\hat{X}],\hat{H}_0]\rangle\right\} \\ &- A(t)^2\langle[[\hat{O},\hat{X}],\hat{X}]\rangle.\end{aligned} \tag{A1}$$

The derivation is straightforward by applying the Ehrenfest theorem to $\mathrm{d}\langle\hat{O}\rangle/\mathrm{d}t$ (see Eq. (14)). Note the appearance of derivatives and quadratic terms of the field. In principle, Eq. (A1) can be used for local control by approximating the derivative of the field by finite differences and solving a quadratic equation for the field. However, the scheme turns out to be very unstable numerically and is not pursued further.

Hence, we now focus on Eq. (16). Since $\mathcal{Y}(t)$ and $\mathcal{Z}(t)$ are complex-valued, the resulting local control expression in Eq. (16) leads to complex-valued fields. This results in a non-Hermitian Hamiltonian and no norm-conserving dynamics. To avoid numerical instabilities, $A(t)$ is made real-valued by modifying it to $[A(t) + A^*(t)]/2$.

Despite those modifications, we still recognized many numerical difficulties. Besides the division by very small $\mathcal{Z}(t)$ and the *ad hoc* introduction of the scaling parameter $\lambda$, only the first time derivative of $\langle O\rangle$ is optimized. For high-frequency fields, this requires very small time steps.

#### a. *"Simple man" optimization*

To remedy this, as another local control algorithm, we introduce here a "simple man" approach where the increase of the expectation value from time $t_0$ to $t_0 + \Delta_t$ is maximized numerically:

$$\max_{A(t_0+\Delta_t/2)} \langle\psi(t_0+\Delta_t)|\hat{O}|\psi(t_0+\Delta_t)\rangle, \tag{A2}$$

where

$$|\psi(t_0+\Delta_t)\rangle = \exp[-\mathrm{i}(\hat{H} + A(t_0+\Delta_t/2)\cdot\hat{X})\Delta_t]|\psi(t_0)\rangle. \tag{A3}$$

This is a simple one-dimensional optimization problem for $A(t_0 + \Delta_t/2)$ that can be solved accurately within about 10 iterations using standard algorithms like Brent's method [1, 2]. While this procedure then requires several propagations per time step, it has the advantage that there are no further parameters and its implementation is straightforward.

In order to avoid too large values and too rapid increases of $A(t)$, the optimization is performed such that $A(t_0 + \Delta_t/2)$ is bounded by

$$A_{\max} \geq |A(t_0+\Delta_t/2)| \leq 2|A(t_0)|, \tag{A4}$$

where $A_{\max}$ is some parameter.

* larsson [at] caltech.e$\delta$u; Present address: Division of Chemistry and Chemical Engineering, California Institute of Technology, Pasadena, CA 91125, USA

#### b. Parameters

For the control expression in Eq. (16), the scaling parameter $\lambda$ was set to 500, $C$ was set to 1 and a maximal allowed absolute value of $A_{\max} = 50$ was taken for the field. The wavefunction was propagated until $T = 15$ (0.36 fs). Clearly, this is a very short propagation time. However, the initial dynamics of the electron ejection is the key to control. For the choice of target, it is much more difficult to control the motion of the electrons when they are already ionized and are located far out in the continuum, compared to when they are still (partially) bounded.

When using Eq. (16), a small time step of $\Delta_t = 0.0125$ was used. The small time step is necessary because the local control expressions are valid only to first order in time [3].

For the "simple man" approach [Eq. (A2)], a larger time step of $\Delta_t = 0.05$ was used. $A_{\max}$ in Eq. (A4) was chosen such that for each time step, the amplitude of the field can only be doubled. Note that this makes the outcome of the optimization dependent on the choice of the time step. Different time steps have been tried.

For the optimizations, we used Eq. (27) for the "simple man" approach and Eq. (28) for the optimization using Eq. (16).

### 2. Derivative-free optimization

The quite restricted functional form of Eq. (35) leads to the occurrence of different maxima on the optimization landscape and the best way to optimize would be to employ global optimization algorithms like evolutionary algorithms [4]. However, since the derivative-free algorithms do not explicitly use gradients, it is conceivable that they avoid getting trapped in local minima. Further, they are robust with respect to a noisy optimization landscape.

In any case, both local and global optimization algorithms were used. As local optimization algorithms, BOBYQA [5] and its cousin COBYLA [6] as implemented in nlopt [7] were used. More sophisticated methods like the "chopped random basis"/CRAB scheme [8–10] were not used.

As a global optimization algorithm, differential evolution, as implemented in SciPy [2] was used. Differential evolution is a special type of evolutionary algorithm. Thus, it is nondeterministic and therefore typically, many separate optimization runs are required in order to get to the (global) optimum. Here, only one run with about 600 iterations was performed. This is because the aim of this study is not to find the *global* maximum but to explore possible fields in order to find interesting mechanisms.

For all optimizations, the propagation time was set to $T = 60$ (1.45 fs).

### 3. Krotov Optimization

When the operator $\hat{O}$ to a projector $\hat{O} = |\phi\rangle\langle\phi|$, the functional $J$ in Eq. (13) becomes

$$J = \langle\psi(T)|\hat{O}|\psi(T)\rangle = |\langle\psi(T)|\,\phi\rangle|^2. \tag{A5}$$

In the Krotov algorithm, the dual function at time $T$ is then formed by

$$\hat{O}|\psi(T)\rangle = \langle\phi|\,\psi(T)\rangle \cdot |\phi\rangle. \tag{A6}$$

This causes a vanishing dual function if $|\langle\phi|\,\psi(T)\rangle|$ approaches 0 which can occur for a bad initial choice of field. To avoid this, we minimized

$$\|\psi(T)-\phi\|^2 = \langle\psi(T)|\,\psi(T)\rangle - \langle\phi|\,\phi\rangle - 2\Re\langle\psi(T)|\,\phi\rangle, \tag{A7}$$

which corresponds to a maximization of $\Re\langle\psi(T)|\,\phi\rangle$ [11]. Then, $|\chi(T)\rangle$ equals $|\phi(T)\rangle$ and there is no trouble with vanishing overlap between the final wavefunction and the target state. Furthermore, this particular goal fixes the global phase of the target.

For all optimizations, we further renormalized the dual function $|\chi(T)\rangle = \hat{O}|\psi(T)\rangle$. This is required because, for bad initial fields, $\hat{O}|\psi(T)\rangle$ has a very small norm. This renormalization essentially corresponds to a decrease of $\lambda_0$ in the Lagrange multiplier (see next paragraph) for the particular iteration.

The Lagrange multiplier for the field constraints was taken as

$$\lambda(t) = \lambda_0 + 100\{\exp(-a_l t) + \exp[-a_l(T-t)]\}, \tag{A8}$$

with $\lambda_0 = 0.03$ and $a_l = 12$. The term with the exponentials ensures that the field starts and ends with negligible values. As mentioned in Section IV B 2, it is crucial to set $A^{\text{ref}}(t)$ to the solution from the previous iteration. Otherwise, it can happen that only $J_3$ [Eq. (24)] is optimized and $\bar{J}$ decreases during the optimization, especially for bad choices of initial fields where $\bar{J} \approx 0$.

### 4. Control of classical dynamics

For the model system introduced in Section II, Hamilton's classical equations of motion (Eq. (26)) take the form of

$$\frac{\mathrm{d}u}{\mathrm{d}t} = p_u/2 - A(t), \qquad \frac{\mathrm{d}v}{\mathrm{d}t} = p_v/2, \tag{A9}$$

$$\frac{\mathrm{d}p_u}{\mathrm{d}t} = -\frac{\partial V(u,v)}{\partial u}, \qquad \frac{\mathrm{d}p_v}{\mathrm{d}t} = -\frac{\partial V(u,v)}{\partial v}. \tag{A10}$$

Those equations were discretized using the fourth-order Runge-Kutta propagator [12]. As control algorithm, we used the black-box collocation-based "optistack" routines from the CasADi [13] software.

The final propagation time was set to $T = 60$ and a time step of $\Delta_t = 0.0024$ was chosen. The initial values

were set to $u(0) = v(0) = 0$ and $p_u(0) = p_v(0) = 0.01$. Nonzero momenta are required in order to initialize the propagation to avoid the system getting trapped at the origin.

To ensure not too large values of the field $A(t)$, an additional term of the form $4\int \mathrm{d}t[A(t)\lambda(t)]^2$ was added to the functional shown in Eq. (36). $\lambda(t)$ is given by Eq. (A8) with $\lambda_0 = 1$ and $a_l = 10$.

### 5. Simulation Method: Dynamically pruned discrete variable representation (DP-DVR)

In the following, the particular method to simulate the TDSE will be described. Double ionization dynamics simulations are very challenging and resource intensive. Besides, the used control optimization methods require *many* successive simulations with very different external fields. It is thus highly important to take great care to select a simulation method that is able to deal with those challenges. The reader who is only interested in the control methodology and/or in the physics may skip this Section.

We represent the wavefunction using a sinc discrete variable representation (DVR) [14, 15] that we symmetrize in the $v$ coordinate; see Section II. Symmetrization is performed by centering the grid around $v = 0$ and using appropriate linear combinations of DVR functions peaked at positive and negative coordinate values. The grid spacing is chosen to be typically about 0.07. To propagate the wavefunction, we employ a short iterative Arnoldi propagator [16, 17] with an accuracy of $10^{-10}$. For the local control propagation, a small coordinate range with grid lengths between 200 and 400 is sufficient as the local control procedure is carried out only for short propagation times; see Section A 1. However, for the other optimization procedures, longer propagation times and with correspondingly larger grid lengths (about 800) are required. This then requires very large basis sizes (overall larger than $10^7$), making the runtime of each propagation very long. Since the control algorithms require many successive propagations, this leads to an unfeasibly long total runtime. To speed up the runtime, we employ our newly developed dynamically pruned DVR (DP-DVR) [18, 19]. There, the sparsity of the wavefunction in coordinate space is exploited. To take into account the spreading and movement of the wavefunction, at each time step new basis functions are added and others are removed. We add new basis functions when the absolute value of the coefficients of the nearest neighbors is larger than about $10^{-8}$. Due to the diagonality of the potential in DVR representation and due to efficient algorithms optimized for orthogonal bases, the pruned DVR outperformed our previously used nonorthogonal phase-space localized von Neumann basis [19, 20]. For details of this procedure, especially the algorithms for the multiplication of the Hamiltonian matrix representation with the wavefunction in the pruned subspace, we refer to Refs. [18, 19]. We further exploit the Toeplitz structure of the operators represented in the sinc DVR; see Ref. [21] for details. Note that only in the $u$ coordinate the DVR bases have operator representations with Toeplitz structure because the symmetrization in $v$ destroys this structure (but gives smaller matrices).

The use of the DP-DVR is crucial to be able to perform many propagations in a small amount of time. For example, a standard fast-Fourier-transform-based [22] propagation with the field from Ref. [20] on a grid with basis size of $4098 \times 4098$ and final propagation time of $T = 450$ took almost two and a half days of runtime on a Nvidia Tesla K80 GPGPU whereas our DP-DVR propagation took about one day of runtime on only six cores of Intel(R) Xeon(R) CPU E5-2650 v2 processors. Furthermore, it should be noted that the performance of DP-DVR heavily depends on the occupancy in coordinate space. For external fields with small intensities that do not lead to major ionization, the propagation takes only minutes to a few hours. However, when major regions in coordinate space are covered, the runtime can be more than two days. This is especially a problem for the Krotov method because for a bad choice of initial field or some operators $\hat{O}$, $|\chi(t)\rangle$ often covers large regions in coordinate space during the backward propagation.

Recently, we have combined dynamical pruning with the multi-configuration time-dependent Hartree (MCTDH) method [23]. While DP-MCTDH could speed up the runtime further, we do not employ it here in order not to increase the complexity of the methodology. For ionization problems, MCTDH is very sensitive to a regularization parameter which controls the level of noise in the wavefunction and has to be given very low values such that low-amplitude ionization can be accurately described. Recent work [24–26] on different ways to regularize the MCTDH equations of motion might decrease this sensitivity.

## Appendix B: Further results for optimization using the Krotov algorithm

We also tried to perform optimizations using the Krotov procedure with a projection operator as target, i.e., $\hat{O} = |\phi\rangle\langle\phi|$. As target states $|\phi\rangle$, we tested several variants of the Gaussian shown in Eq. (29); we also used parts of a wavefunction extracted from a propagation with initial fields that lead to some occupancy in region $D_1$. We further tested a target state that extracts parts of the current wavefunction ($|\psi^{(p)}(T)\rangle$ at iteration $p$) from region $D_1$. However, with the aforementioned targets we were not able to optimize the population in region $D_1$ compared to region $D_2$. Besides numerical instabilities, both regions are always occupied, even after the Krotov optimization has reached a plateau.

To guide the Krotov algorithm, additionally, we tested target operators of the form $\hat{O} = |\phi_1\rangle\langle\phi_1| - |\phi_2\rangle\langle\phi_2|$, where $|\phi_2\rangle$ is located in region $D_2$. This corresponds

to a min-max optimization. Note that this operator is not positive and as such, the Krotov algorithm is not monotonically convergent, although there are ways to retain monotonicity [27]. Even with that target, we were not successful in finding appropriate fields that lead to a significant occupancy in region $D_1$, compared to region $D_2$. This might be due to inappropriately chosen target states. After the propagation with typical fields, the wavefunction never has simple Gaussian-like shapes and also extracting parts of the wavefunction is unphysical as this assumes that the parts that are not extracted are negligible.


[1] W. H. Press, S. A. Teukolsky, W. T. Vetterling, and B. P. Flannery, *Numerical Recipes*, 3rd ed. (Cambridge University Press, 2007).

[2] E. Jones, T. Oliphant, P. Peterson, *et al.*, "SciPy: Open source scientific tools for Python," (2001).

[3] This could be improved by higher-order discretizations of the time evolution.

[4] T. Weise, *Global Optimization Algorithms*, 3rd ed. (`www.it-weise.de`, 2011).

[5] M. J. D. Powell, Cambridge NA Report NA200906 (2009).

[6] M. J. D. Powell, Acta Numer. **7**, 287–336 (1998).

[7] S. G. Johnson, "The nlopt nonlinear-optimization package," `http://ab-initio.mit.edu/nlopt` (2018).

[8] N. Rach, M. M. Müller, T. Calarco, and S. Montangero, Phys. Rev. A **92**, 062343 (2015).

[9] T. Caneva, T. Calarco, and S. Montangero, Phys. Rev. A **84**, 022326 (2011).

[10] P. Doria, T. Calarco, and S. Montangero, Phys. Rev. Lett. **106**, 190501 (2011).

[11] J. Werschnik and E. K. U. Gross, J. Phys. B **40**, R175 (2007).

[12] P. Deuflhard and F. Bornemann, *Numerische Mathematik 2: Gewöhnliche Differentialgleichungen*, 3rd ed. (de Gruyter, 2008).

[13] J. A. E. Andersson, J. Gillis, G. Horn, J. B. Rawlings, and M. Diehl, Math. Prog. Comp. **11**, 1 (2019).

[14] D. T. Colbert and W. H. Miller, J. Chem. Phys. **96**, 1982 (1992).

[15] D. J. Tannor, *Introduction to Quantum Mechanics: A Time-Dependent Perspective*, 1st ed. (University Science Books, 2007).

[16] T. J. Park and J. C. Light, J. Chem. Phys. **85**, 5870 (1986).

[17] M. H. Beck, A. Jäckle, G. A. Worth, and H.-D. Meyer, Phys. Rep. **324**, 1 (2000).

[18] H. R. Larsson, B. Hartke, and D. J. Tannor, J. Chem. Phys. **145**, 204108 (2016).

[19] D. J. Tannor, S. Machnes, E. Assémat, and H. R. Larsson, "Phase space vs. coordinate space methods: Prognosis for large quantum calculations," in *Advances in Chemical Physics*, Vol. 163 (John Wiley & Sons, Inc., 2018) pp. 273–323.

[20] E. Assémat, S. Machnes, and D. Tannor, "Double ionization of Helium from a phase space perspective," (2015), arXiv:1502.05165.

[21] H. R. Larsson, J. Riedel, J. Wei, F. Temps, and B. Hartke, J. Chem. Phys. **148**, 204309 (2018).

[22] D. Kosloff and R. Kosloff, J. Comp. Phys. **52**, 35 (1983).

[23] H. R. Larsson and D. J. Tannor, J. Chem. Phys. **147**, 044103 (2017).

[24] H.-D. Meyer and H. Wang, J. Chem. Phys. **148**, 124105 (2018).

[25] B. Kloss, I. Burghardt, and C. Lubich, J. Chem. Phys. **146**, 174107 (2017).

[26] U. Manthe, J. Chem. Phys. **142**, 244109 (2015).

[27] D. M. Reich, M. Ndong, and C. P. Koch, J. Chem. Phys. **136**, 104103 (2012).
